# Supplementary material for: Photoemission Spectroscopy and Orbital Imaging from Koopmans-Compliant Functionals
Source: arXiv:1409.4210 source file (2014-09-15)
Supplement: Supplementary file 1 [file Supplemental_Material.pdf]

# Supplemental material to "Photoemission Spectroscopy and Orbital Imaging from Koopmans-Compliant Functionals"

Ngoc Linh Nguyen,[1] Giovanni Borghi,[1] Andrea Ferretti,[2] Ismaila Dabo,[3] and Nicola Marzari[1]

[1] *Theory and Simulations of Materials (THEOS), and National Center for Computational Design and Discovery of Novel Materials (MARVEL), École Polytechnique Fédérale de Lausanne, 1015 Lausanne, Switzerland*

[2] *Centro S3, CNR–Istituto Nanoscienze, I-41125 Modena, Italy*

[3] *Department of Materials Science and Engineering, Materials Research Institute, and Penn State Institutes of Energy and the Environment, The Pennsylvania State University, University Park, PA 16802, USA*

(Dated: August 29, 2014)

## TECHNICAL DETAILS

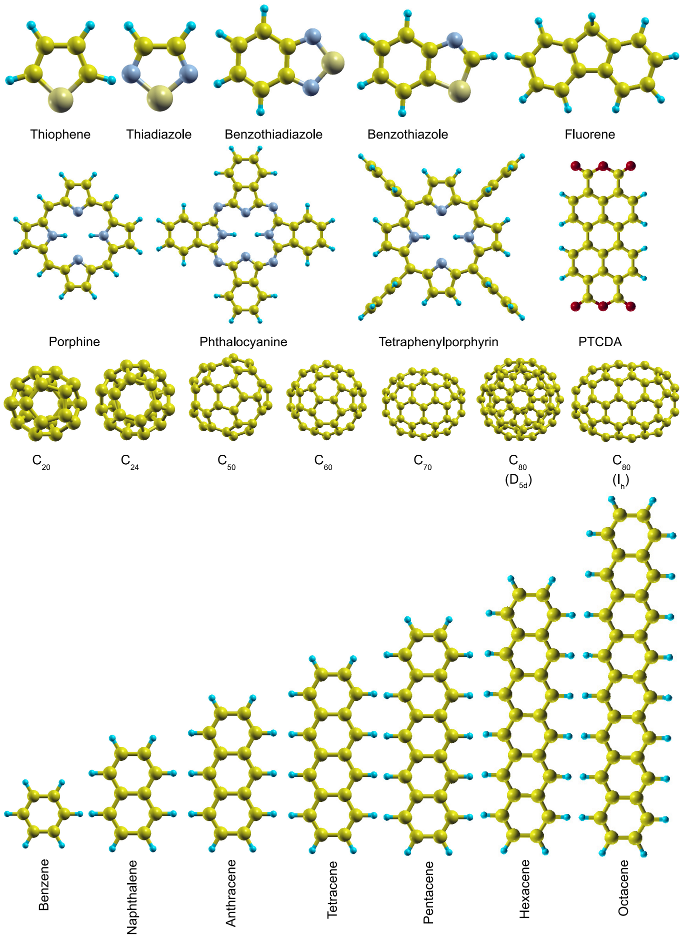


FIG. 1. Representative sample of organic photovoltaic molecules for benchmarking the performance of electronic-structure methods.

In this work, we carry out calculations on several organic molecules relevant to photovoltaic junctions. We can group them in three sets: (i) molecules which constitute elemental components for relevant photovoltaic organics, (ii) fullerenes, and (iii) acenes. Their names and geometries are presented in Fig. 1. The UPS calculations are set up for molecules in their gas phase. We place them inside an orthorhombic cell with 18 Bohr of vacuum separating periodic replicas, sufficient to converge total energy and electronic eigenvalues, the Coulomb interaction between periodic images being suppressed by means of reciprocal space counter-charge corrections [1]. Molecular geometries are optimized via Kohn-Sham DFT, with the Perdew-Burke-Ernzerhof (PBE) [2] approximation for the exchange-correlation functional. The electron-ion interactions are computed using norm-conserving pseudopotentials [3], and the energy cutoff for the plane wave expansion is set to 60 Ry (240 Ry for the charge density cutoff).

In order to compute electronic properties consistent with the optimized geometries, all orbital density dependent (ODD) calculations (either Perdew-Zunger (PZ) self-interaction correction method or Koopmans-compliant functionals, e.g. KI or KIPZ) presented here and in the main letter are also computed on top of the PBE functional. All calculations are spin resolved. The combination of PZ and KIPZ with PBE as base functional was shown to give the best results for the electronic eigenvalue spectrum when minimized on the Hilbert space of complex wave functions [4, 5], which we therefore use here as basis set.

The excellent performance of Koopmans-compliant functionals to predict the first ionization potential (IP) and electron affinity (EA) energy levels has been shown in the main Letter through Table I and Figure 2. The IP and EA predictions for each single molecule are displayed in Table I and II.

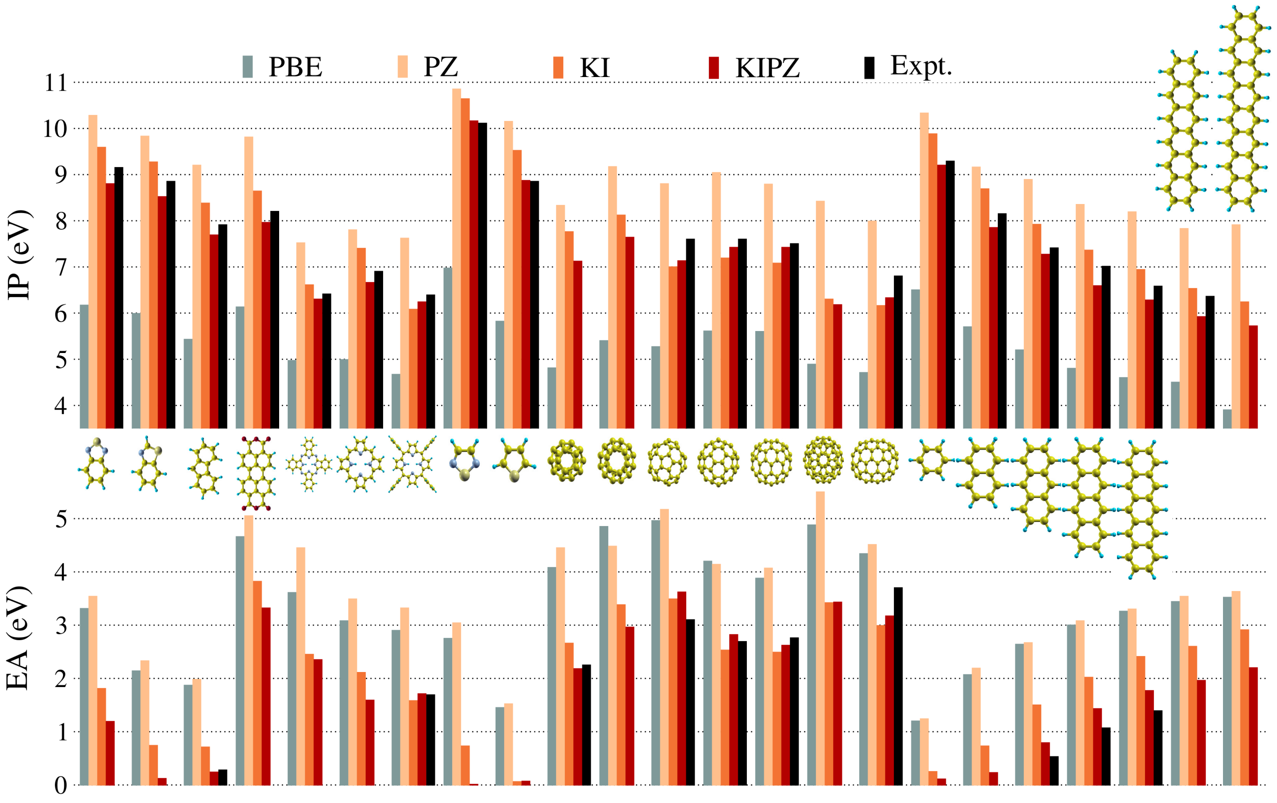


FIG. 2. PBE, PZ, KI, and KIPZ ionization potentials (IPs) and electron affinities (EAs) of organic photovoltaic molecules, compared with experiments, when available.

## ULTRAVIOLET PHOTOEMISSION SPECTROSCOPY

In this section we provide more details concerning the simulation of ultra-photoemission (UPS) spectra within the one-step model of photoemission. UPS simulations are carried out as a post-processing of electronic structure calculations with the Quantum ESPRESSO plane-wave pseudopotential code [29]. Each UPS simulation involves: (i) computing the generalized electronic density of states (GDOS) of valence states, which depends on the binding energy of the excited electron, on the energy of the incoming photon ($h\nu$), and on the kinetic energy of the emitted photoelectron $E_{\rm kin}$; and (ii) correcting the photoemission intensity of GDOS via the photoionization cross-section for each wave function. In all PBE calculations shown in this work we use KS orbitals, $\{\varphi_i(\boldsymbol{r})\}$ and corresponding eigenvalues, $\{\varepsilon_i\}$ as approximations for Dyson orbitals and their binding energies, respectively, while we use canonical orbitals [5] and their generalized eigenvalues in the case of orbital-density dependent calculations (PZ, KI, KIPZ).

The photoionization with the quantum of energy $h\nu$ excites one electron, having mass $m$, from a bound state $\varphi_i(\boldsymbol{r})$ to an unbound state whose energy and momentum are read by the detector. We approximate this unbound state with a plane wave:

$$\xi_{\boldsymbol{k}}(\boldsymbol{r}) = \sqrt{\frac{1}{V}}\,\exp(i\boldsymbol{k}\cdot\boldsymbol{r})\,, \tag{1}$$

normalized in a large cubic box of volume $V$, and with energy equal to ($k = |\boldsymbol{k}|$)

$$E_{\rm kin} = \frac{\hbar^2 k^2}{2m}.$$

We can now rewrite the summation in Eq. (2) of the main Letter as:

$$I^\nu = \sum_{\boldsymbol{k}} I^\nu_{\boldsymbol{k}}\,, \tag{2}$$

TABLE I. Ionization energies of several photovoltaic molecules computed with PBE, PZ, Koopmans functionals and scf-GW, compared to experiment, when available.

| | PBE | PZ | KI | KIPZ | scf-GW | Expt. |
|---|---|---|---|---|---|---|
| Benzothiadiazole | 6.17 | 10.28 | 9.59 | 8.8 | 8.56 [a] | 9.15 [b] |
| Benzothiazole | 5.99 | 9.83 | 9.27 | 8.52 | 8.48 [a] | 8.85 [c] |
| Fluorene | 5.43 | 9.2 | 8.38 | 7.69 | 7.64 [a] | 7.91 [d] |
| PTCDA | 6.13 | 9.81 | 8.64 | 7.96 | 7.68 [a] | 8.2 [e] |
| Phthalocyanine | 4.97 | 7.52 | 6.61 | 6.3 | 6.1 [a] | 6.41 [f] |
| Porphine | 4.99 | 7.8 | 7.4 | 6.66 | 6.7 [a] | 6.9 [g] |
| Tetraphenylporphyrin | 4.67 | 7.62 | 6.08 | 6.24 | 6.2 [a] | 6.39 [h] |
| Thiadiazole | 6.97 | 10.85 | 10.64 | 10.16 | 9.89 [a] | 10.11 [i] |
| Thiophene | 5.82 | 10.15 | 9.52 | 8.87 | 8.63 [a] | 8.85 [j] |
| $C_{20}$ | 4.81 | 8.33 | 7.76 | 7.12 | 7.41 [k] | |
| $C_{24}$ | 5.4 | 9.17 | 8.12 | 7.64 | 7.81 [k] | |
| $C_{50}$ | 5.27 | 8.8 | 7 | 7.13 | 7.35 [k] | 7.6 [l] |
| $C_{60}$ | 5.61 | 9.04 | 7.19 | 7.42 | 7.41 [a] | 7.6 [l] |
| $C_{70}$ | 5.6 | 8.79 | 7.08 | 7.42 | 7.45 [k] | 7.5 [m] |
| $C_{80}(D_{5d})$ | 4.89 | 8.42 | 6.3 | 6.18 | 6.65 [k] | |
| $C_{80}(I_h)$ | 4.71 | 7.99 | 6.16 | 6.33 | 6.95 [k] | 6.8 [l] |
| Benzene | 6.5 | 10.33 | 9.88 | 9.2 | | 9.29 [n] |
| Naphthalene | 5.7 | 9.16 | 8.69 | 7.85 | | 8.15 [o] |
| Anthracene | 5.2 | 8.89 | 7.92 | 7.27 | 7.06 [a] | 7.41 [o] |
| Tetracene | 4.8 | 8.35 | 7.36 | 6.59 | 6.51 [a] | 7.01 [o] |
| Pentacene | 4.6 | 8.19 | 6.94 | 6.28 | 6.12 [a] | 6.58 [o] |
| Hexacene | 4.5 | 7.83 | 6.53 | 5.92 | | 6.36 [o] |
| Octacene | 3.9 | 7.91 | 6.24 | 5.72 | | |

[a] Ref. 6
[b] Ref. 7
[c] Ref. 8
[d] Ref. 9
[e] Ref. 10
[f] Ref. 11
[g] Ref. 12
[h] Ref. 13
[i] Ref. 14
[j] Ref. 15
[k] Ref. 16
[l] Ref. 17
[m] Ref. 18
[n] Ref. 19
[o] Ref. 20

decomposing the photoemission intensity in components depending on the wave vector of the photoelectron, each equal to

$$I^{\nu}_{\boldsymbol{k}} = \mathcal{N} \sum_i |\boldsymbol{A} \cdot \boldsymbol{P}_{i,\boldsymbol{k}}|^2 \times \delta \left( h\nu - \varepsilon_i - \frac{\hbar^2 k^2}{2m} \right), \tag{3}$$

where $\mathcal{N}$ is a normalization factor for the spectrum, and

$$\boldsymbol{P}_{i,\boldsymbol{k}} = -i\hbar \langle \varphi_i | \nabla_{\boldsymbol{r}} | \xi_{\boldsymbol{k}} \rangle. \tag{4}$$

In order to take into account the random orientations of molecules in the gas phase, we need to average $I^{\nu}_{\boldsymbol{k}}$ over all incoming photon directions, and average it over outgoing photoelectron directions [30]. The first averaging is done by

TABLE II. Electron affinities of several photovoltaic molecules computed with PBE, PZ, Koopmans functionals and scf-GW, compared to experiment, when available.

| | PBE | PZ | KI | KIPZ | scf-GW | Expt. |
|---|---|---|---|---|---|---|
| Benzothiadiazole | 3.31 | 3.54 | 1.81 | 1.19 | 0.42 [a] | |
| Benzothiazole | 2.14 | 2.33 | 0.74 | 0.12 | -0.92 [a] | |
| Fluorene | 1.87 | 1.98 | 0.71 | 0.24 | -0.74 [a] | 0.28 [b] |
| PTCDA | 4.66 | 5.05 | 3.82 | 3.32 | 2.68 [a] | |
| Phthalocyanine | 3.61 | 4.45 | 2.45 | 2.35 | 2.07 [a] | |
| Porphine | 3.08 | 3.49 | 2.11 | 1.59 | 1.39 [a] | |
| Tetraphenylporphyrin | 2.9 | 3.32 | 1.58 | 1.71 | 1.49 [a] | 1.69 [c] |
| Thiadiazole | 2.75 | 3.04 | 0.73 | 0.01 | -0.92 [a] | |
| Thiophene | 1.45 | 1.52 | 0.06 | 0.07 | -1.98 [a] | |
| $C_{20}$ | 4.08 | 4.45 | 2.66 | 2.18 | 2.36 [d] | 2.25 [e] |
| $C_{24}$ | 4.85 | 4.48 | 3.38 | 2.96 | 2.88 [d] | |
| $C_{50}$ | 4.96 | 5.17 | 3.49 | 3.62 | 3.73 [d] | 3.1 [f] |
| $C_{60}$ | 4.2 | 4.14 | 2.53 | 2.82 | 2.5 [a] | 2.69 [g] |
| $C_{70}$ | 3.88 | 4.07 | 2.49 | 2.62 | 2.83 [d] | 2.76 [h] |
| $C_{80}(D_{5d})$ | 4.88 | 5.5 | 3.42 | 3.43 | 3.88 [d] | 3.7 [f] |
| $C_{80}(I_h)$ | 4.34 | 4.51 | 2.99 | 3.17 | 4.38 [d] | |
| Benzene | 1.2 | 1.24 | 0.25 | 0.11 | | |
| Naphthalene | 2.07 | 2.19 | 0.73 | 0.23 | | |
| Anthracene | 2.64 | 2.67 | 1.5 | 0.79 | 0.32 [a] | 0.53 [i] |
| Tetracene | 3 | 3.08 | 2.02 | 1.43 | 0.93 [a] | 1.07 [j] |
| Pentacene | 3.26 | 3.3 | 2.41 | 1.77 | 1.36 [a] | 1.39 [j] |
| Hexacene | 3.44 | 3.54 | 2.6 | 1.96 | | |
| Octacene | 3.52 | 3.63 | 2.91 | 2.2 | | |

[a] Ref. 6
[b] Ref. 21
[c] Ref. 22
[d] Ref. 16
[e] Ref. 23
[f] Ref. 24
[g] Ref. 25
[h] Ref. 26
[i] Ref. 27
[j] Ref. 28

integrating over the solid angle ($d\Omega_{\rm ph} = \sin\theta d\theta\, d\phi$) the direction of the incoming radiation,

$$\bar{I}^{\nu}_{\boldsymbol{k}} = \mathcal{N} \sum_i \delta\left(h\nu - \varepsilon_i - \frac{\hbar^2 k^2}{2m}\right) \times \frac{1}{4\pi} \int |\boldsymbol{A} \cdot \boldsymbol{P}_{i,\boldsymbol{k}}|^2 d\Omega_{\rm ph}\,. \tag{5}$$

Since UPS experiments are usually carried out with unpolarized light, we need to average Eq.(5) also over the polarization of the incident photon. Parametrizing the electro-magnetic vector potential as $\boldsymbol{A} = A\boldsymbol{u}$, we find the decomposition:

$$|\boldsymbol{u} \cdot \boldsymbol{P}_{i,\boldsymbol{k}}|^2 = \frac{1}{2}(|\boldsymbol{u}_1 \cdot \boldsymbol{P}_{i,\boldsymbol{k}}|^2 + |\boldsymbol{u}_2 \cdot \boldsymbol{P}_{i,\boldsymbol{k}}|^2), \tag{6}$$

where $\boldsymbol{u}_1$ and $\boldsymbol{u}_2$ are the two polarization directions perpendicular to the photon propagation vector, $\boldsymbol{k}_{\rm ph}$. These three vectors form a right-hand chiral system of axes, so that:

$$|\boldsymbol{P}_{i,\boldsymbol{k}}|^2 = |\boldsymbol{u}_1 \cdot \boldsymbol{P}_{i,\boldsymbol{k}}|^2 + |\boldsymbol{u}_2 \cdot \boldsymbol{P}_{i,\boldsymbol{k}}|^2 + \frac{|\boldsymbol{k}_{\rm ph} \cdot \boldsymbol{P}_{i,\boldsymbol{k}}|^2}{|\boldsymbol{k}_{\rm ph}|^2}\,. \tag{7}$$

Eq. (5) can then be written as:

$$\begin{aligned}\bar{I}^{\nu}_{\boldsymbol{k}} &= \mathcal{N}\sum_i \delta\left(h\nu - \varepsilon_i - \frac{\hbar^2 k^2}{2m}\right) \times \frac{A^2}{4\pi}\int\left(|\boldsymbol{P}_{i,\boldsymbol{k}}|^2 - \frac{|\boldsymbol{k}_{\rm ph}\cdot\boldsymbol{P}_{i,\boldsymbol{k}}|^2}{|\boldsymbol{k}_{\rm ph}|^2}\right)d\Omega_{\rm ph} \\ &= \mathcal{N}\sum_i \delta\left(h\nu - \varepsilon_i - \frac{\hbar^2 k^2}{2m}\right) \times \frac{A^2|\boldsymbol{P}_{i,\boldsymbol{k}}|^2}{2}\int(1-\cos^2\theta_{\rm ph})d[\cos(\theta_{\rm ph})] \\ &= \mathcal{N}\sum_i \delta\left(h\nu - \varepsilon_i - \frac{\hbar^2 k^2}{2m}\right) \times \frac{2A^2|\boldsymbol{P}_{i,\boldsymbol{k}}|^2}{3}.\end{aligned} \tag{8}$$

We see therefore that the first averaging results only in a factor of 2/3, which can be adsorbed in the renormalization $\mathcal{N}$ of the photoemission spectrum.

In order to perform the averaging over photoelectron directions, we first write $\varphi_i(\boldsymbol{r})$ in terms of its plane-wave coefficients in Fourier space:

$$\varphi_i(\boldsymbol{r}) = \sum_{\boldsymbol{G}} \tilde{\varphi}_i(\boldsymbol{G})\exp(i\boldsymbol{G}\cdot\boldsymbol{r}), \tag{9}$$

so that $\boldsymbol{P}_{i,\boldsymbol{k}}$ can be obtained, operatively, from the following summation

$$\boldsymbol{P}_{i,\boldsymbol{k}} = \hbar\boldsymbol{k}\sum_{\boldsymbol{G}}\tilde{\varphi}_i(\boldsymbol{G})\delta(\boldsymbol{G}-\boldsymbol{k}). \tag{10}$$

We next compute the sum on a spherical shell of radius $k$

$$\bar{I}^{\nu}_{\boldsymbol{k}} \to \bar{I}^{\nu}_{k} = \mathcal{N}\hbar^2 k^2 \sum_i \delta\left(h\nu - \varepsilon_i - \frac{\hbar^2 k^2}{2m}\right)\sum_{\boldsymbol{G}}|\tilde{\varphi}_i(\boldsymbol{G})|^2\delta(G-k). \tag{11}$$

The first delta function in Eq. (11) imposes energy conservation, while the second one imposes momentum conservation in a gas-phase photoemission process in which all directions for the outgoing electron are equivalent. In practical calculations, both delta functions can be represented as a Lorentzian distribution of finite width:

$$\delta(h\nu - \varepsilon_i - E_{\rm kin}) \approx \frac{\Gamma_h}{2\pi[(h\nu - \varepsilon_i - E_{\rm kin})^2 + \Gamma_h^2]} \tag{12}$$

and

$$\delta(G-k) \approx \frac{\Gamma_g}{2\pi[(G-k)^2 + \Gamma_g^2]}\,, \tag{13}$$

where $\Gamma_h$ is the inverse lifetime of the hole created by the photoemission process. In our work $\Gamma_h$ is chosen so as to minimize the difference in the areas between theoretical and experimental spectra, whenever these are available. In the absence of experimental spectra, it is set to 0.3 eV (which is the parameter we fit from the HeI $C_{70}$ experimental photoemission spectrum). In contrast, $\Gamma_g$ is set equal to the resolution of the plane-wave grid used in each calculation.

The quantity $\bar{I}^{\nu}_{k}$ in Eq. (11) is the photoemission intensity as a function of photon energy ($h\nu$) and the kinetic energy of the ejected electron [$\hbar^2k^2/(2m)$]. In the main Letter we show the accuracy of this model for photoemission when used on top of electronic structure calculations with Koopmans-compliant functionals for three selected molecules. In this supporting information, we provide extra theoretical UPS (compared to experimental data when available) computed with KIPZ and shown in Fig. 3. The quantity presented in all photoemission figures is $\bar{I}^{\nu}_{k}$, plotted for a given $\nu$ as a function of the binding energy of the electron, which is identical to the difference $E_b = h\nu - \hbar^2k^2/(2m)$. In practice, the averaged photoemission intensity in Eq. (11) is displayed as a function of the variables $E_b$ and $\nu$ as

$$\bar{I}^{\nu}_{E_b} = \mathcal{N}\hbar^2 A^2 k^2 \sum_i \delta(E_b - \varepsilon_i)\sum_{\boldsymbol{G}}|\tilde{\varphi}_i(\boldsymbol{G})|^2\delta(G-k), \tag{14}$$

where the modulus of the wave vector $\boldsymbol{k}$ is uniquely determined from $\nu$ and $E_b$ as

$$k = \sqrt{\frac{2m}{\hbar^2}(h\nu - E_b)}.$$

The values of incoming photon energy $h\nu$ are specified in each spectral plot, while the normalization $\mathcal{N}$ is chosen so as to make the intensity of the highest peak of each spectrum equal to one.

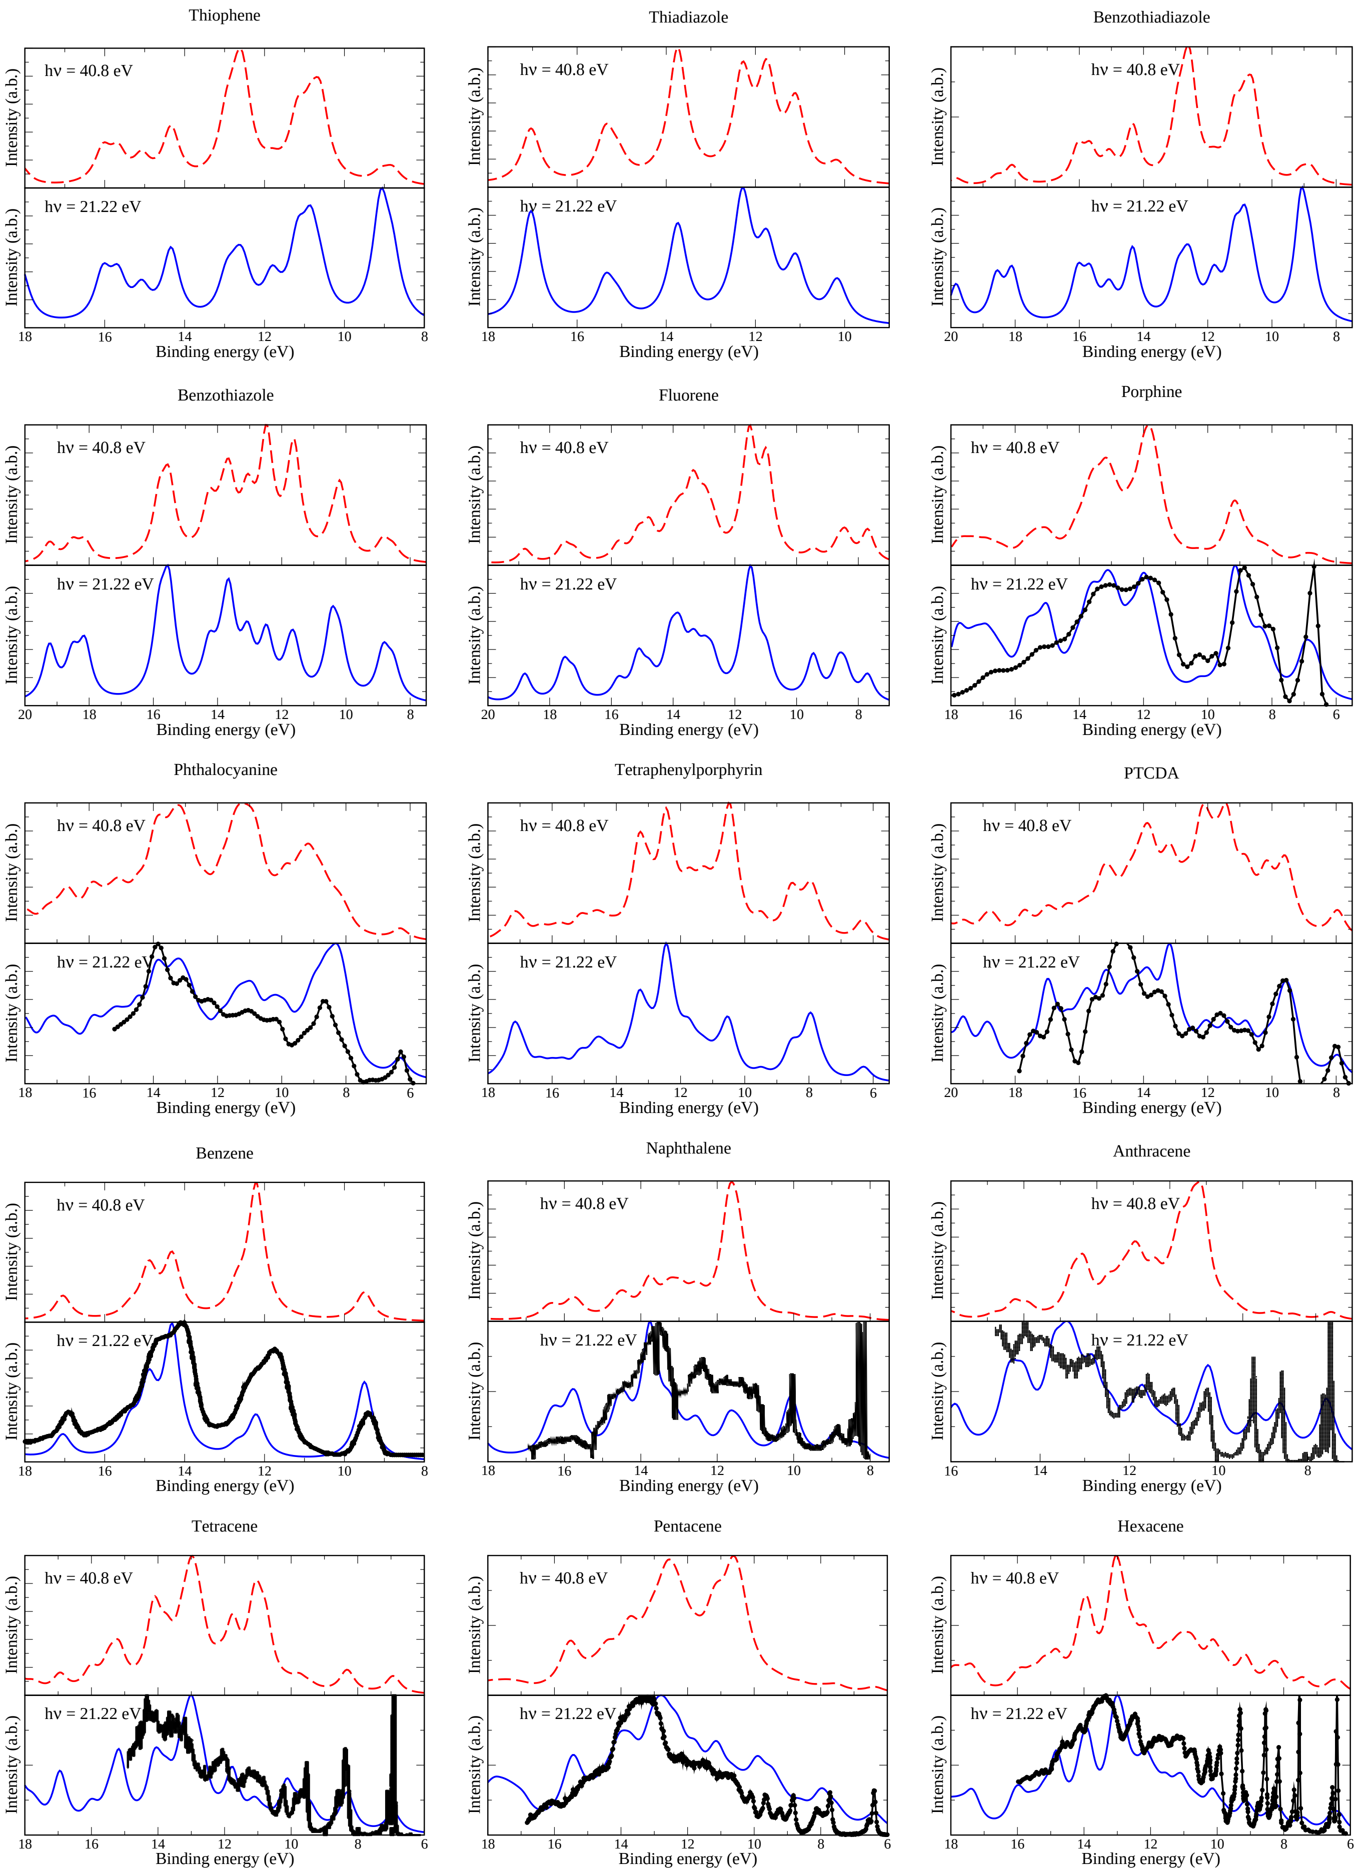
Thiophene
Thiadiazole
Benzothiadiazole
Benzothiazole
Fluorene
Porphine
Phthalocyanine
Tetraphenylporphyrin
PTCDA
Benzene
Naphthalene
Anthracene
Tetracene
Pentacene
Hexacene
hν = 40.8 eV
hν = 21.22 eV
Intensity (a.b.)
Binding energy (eV)

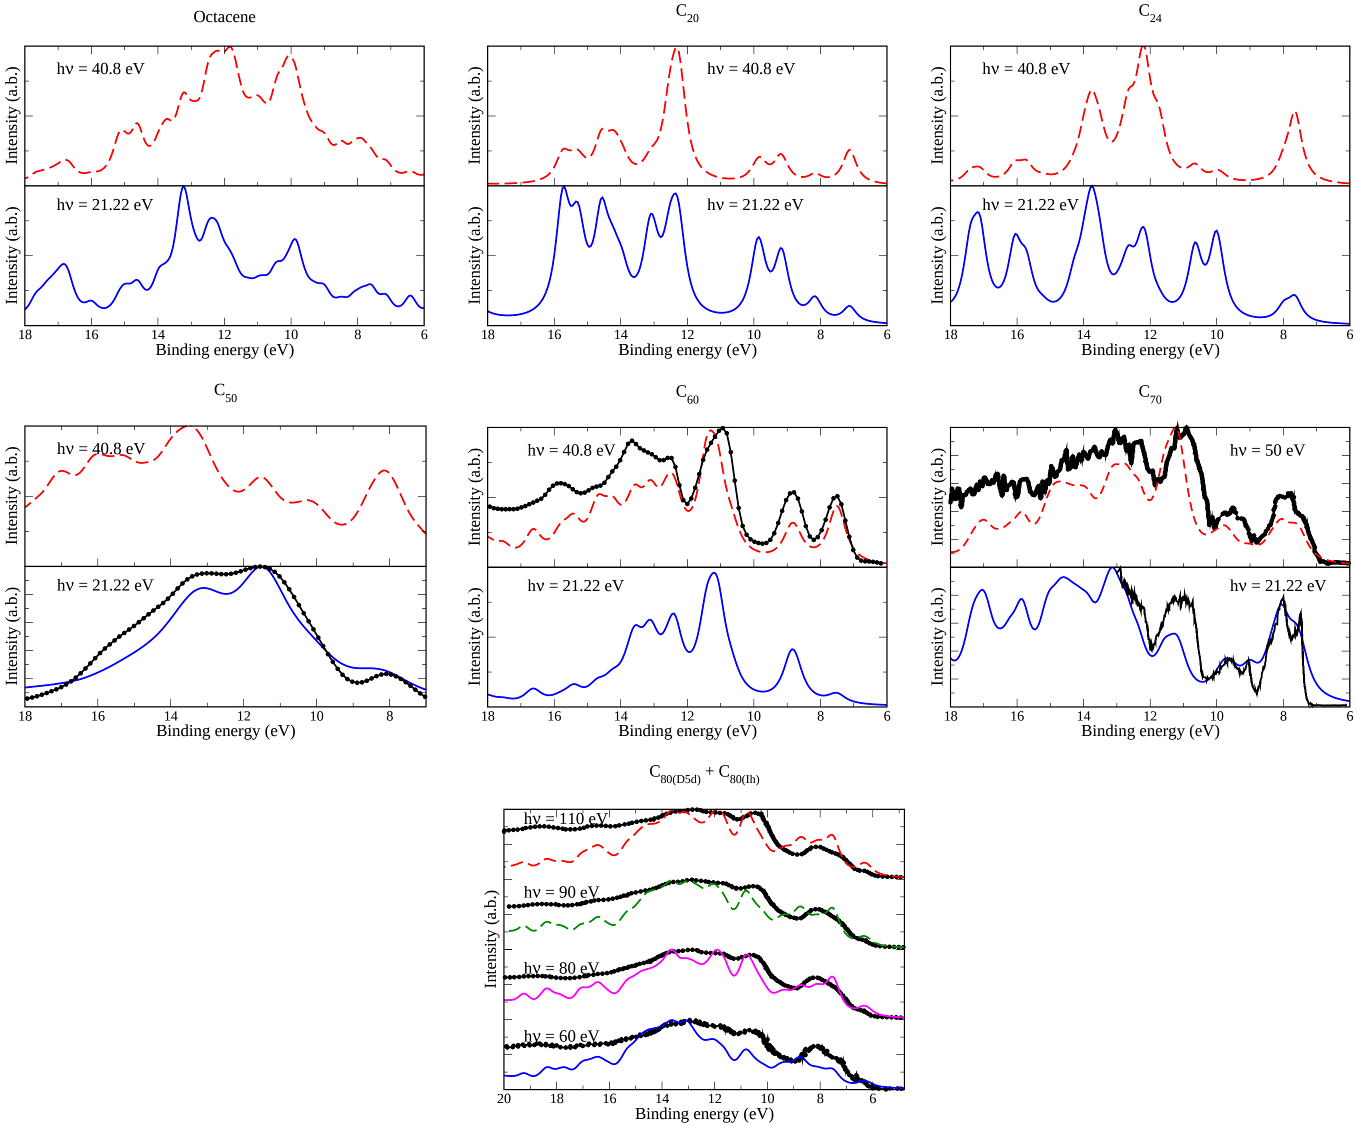


FIG. 3. UPS computed with KIPZ for the photovoltaic organic molecules shown in Fig. 1, simulated for different incoming photon energies ($h\nu$). Theoretical spectra are compared with the available gas phase experimental data measured at the same photon energy (black dotted-line). Experimental data are taken from Ref. [12] for porphine, Ref. [11] for phthalocyanine, Ref. [10] for PTCDA, Ref. [31] for benzene, Ref. [32] for naphthalene, Ref. [33] for anthracene, tetracene, and pentacene, Ref. [34] for hexacene, Ref. [35] for fullerenes $C_{60}$ and Refs. [18] and [35] for fullerenes $C_{70}$, while the data for fullerenes $C_{50}$ and $C_{80}$ are taken from UPS measurements on thin films [36] and in the bulk-phase [37], respectively.

## ORBITAL TOMOGRAPHY MOMENTUM MAPS

As discussed in the main Letter, angular-resolved photoemission (ARPES) experimental data can be connected to molecular orbital maps in momentum space. This enables to compare theoretical and experimental predictions at the level of each eigenstate of a system, a procedure which provides an enormous insight into the electronic structure of a system.

From Eq. (3), the ARPES momentum map can be modeled by projecting on a plane (e.g., $[k_x, k_y]$) the UPS intensity of a semi-spherical shell in photoelectron momentum space, of square radius determined by its kinetic energy:

$$I^{\nu}_{k_x,k_y,\frac{\hbar^2k^2}{(2m)}} = \mathcal{N}\hbar^2 \sum_{i,k_z} \left|\langle\varphi_i|\boldsymbol{A}\cdot\nabla_{\boldsymbol{r}}|\xi_{\boldsymbol{k}}\rangle\right|^2 \times \delta\left(h\nu - \varepsilon_i - \frac{\hbar^2k^2}{(2m)}\right). \qquad (15)$$

From the above expression one sees that the photoemission intensity is proportional to the Fourier transform of the

Dyson orbital corrected by the polarization factor $\boldsymbol{A}\cdot\boldsymbol{k}$:

$$I^{\nu}_{k_x,k_y,\frac{\hbar^2k^2}{(2m)}} = \mathcal{N}\hbar^2 \sum_{i,k_z} |\tilde{\varphi}(k_x,k_y)|^2 \times |\boldsymbol{A}\cdot\boldsymbol{k}|^2 \delta\left(h\nu - \varepsilon_i - \frac{\hbar^2k^2}{(2m)}\right). \tag{16}$$

Since ARPES measurements are usually performed on surface-adsorbed molecules, one is able to define precisely the orientation of the molecule with respect to the directions of incoming photon and outgoing photoelectron. This means that the factor $|\boldsymbol{A}\cdot\boldsymbol{k}|^2$ can be known experimentally, and the Fourier transforms of molecular orbitals can be extracted from the photoemission data [38] and compared to theoretical momentum maps. Again, $I^{\nu}_{k_x,k_y,\frac{\hbar^2k^2}{(2m)}}$ can be written alternatively as $I^{\nu}_{k_x,k_y,E_b}$, thus allowing to define for each value of $E_b$ an intensity map in momentum space.

---


[1] Y. Li and I. Dabo, Phys. Rev. B **84**, 155127 (2011).
[2] J. P. Perdew, K. Burke, and M. Ernzerhof, Physical Review Letters **77**, 3865 (1996).
[3] The norm-conserving pseudopotentials for C, O, S, N and H were taken from Quantum ESPRESSO pseudopotential download page: http://www.quantum-espresso.org/pseudo.php.
[4] S. Klüpfel, P. Klüpfel, and H. Jónsson, Physical Review A **84**, 050501 (2011).
[5] G. Borghi, A. Ferretti, N. L. Nguyen, I. Dabo, and N. Marzari, Phys. Rev. B **90**, 075135 (2014).
[6] X. Blase, C. Attaccalite, and V. Olevano, Physical Review B **83**, 115103 (2011).
[7] R. A. W. Johnstone and F. A. Mellon, Journal of the Chemical Society, Faraday Transactions 2: Molecular and Chemical Physics **69**, 1155 (1973).
[8] G. Salmona, R. Faure, and E.-J. Vincent, C.R. Acad. Sci. Ser. 3 **280**, 605 (1975).
[9] B.Ruščić, B. Kovač, L. Klasinc, and H. Güsten, Zeitschrift für Naturforschung A **33**, 1006 (1978).
[10] N. Dori, M. Menon, L. Kilian, M. Sokolowski, L. Kronik, and E. Umbach, Physical Review B **73**, 195208 (2006).
[11] J. Berkowitz, The Journal of Chemical Physics **70**, 2819 (1979).
[12] P. Dupuis, R. Roberge, and C. Sandorfy, Chemical Physics Letters **75**, 434 (1980).
[13] S. C. Khandelwal and J. L. Roebber, Chemical Physics Letters **34**, 355 (1975).
[14] T. Pasinszki, M. Krebsz, and G. Vass, Journal of Molecular Structure **966**, 85 (2010).
[15] M. Bajić, K. Humski, L. Klasinc, and B. Ruščić, Zeitschrift fr Naturforschung B **40**, 1214 (1985).
[16] M. L. Tiago, P. R. C. Kent, R. Q. Hood, and F. A. Reboredo, The Journal of Chemical Physics **129**, 084311 (2008).
[17] J. A. Zimmerman, J. R. Eyler, S. B. H. Bach, and S. W. McElvany, The Journal of Chemical Physics **94**, 3556 (1991).
[18] D. L. Lichtenberger, M. E. Rempe, and S. B. Gogosha, Chemical Physics Letters **198**, 454 (1992).
[19] M. N. Piancastelli, M. K. Kelly, Y. Chang, J. T. McKinley, and G. Margaritondo, Physical Review B **35**, 9218 (1987).
[20] D. Biermann and W. Schmidt, Journal of the American Chemical Society **102**, 3163 (1980).
[21] L. Wojnrovits and G. Fldik, Journal of Chromatography A **234**, 451 (1982).
[22] H. L. Chen, Y. H. Pan, S. Groh, T. E. Hagan, and D. P. Ridge, Journal of the American Chemical Society **113**, 2766 (1991).
[23] H. Prinzbach, F. Wahl, A. Weiler, P. Landenberger, J. Wrth, L. T. Scott, M. Gelmont, D. Olevano, F. Sommer, and B. von Issendorff, Chemistry A European Journal **12**, 62686280 (2006).
[24] S. Yang, C. Pettiette, J. Conceicao, O. Cheshnovsky, and R. Smalley, Chemical Physics Letters **139**, 233 (1987).
[25] X.-B. Wang, C.-F. Ding, and L.-S. Wang, The Journal of Chemical Physics **110**, 8217 (1999).
[26] X.-B. Wang, H.-K. Woo, X. Huang, M. M. Kappes, and L.-S. Wang, Physical Review Letters **96**, 143002 (2006).
[27] J. Schiedt and R. Weinkauf, Chemical Physics Letters **266**, 201 (1997).
[28] L. Crocker, T. Wang, and P. Kebarle, Journal of the American Chemical Society **115**, 7818 (1993).
[29] P. Giannozzi, S. Baroni, N. Bonini, M. Calandra, R. Car, C. Cavazzoni, D. Ceresoli, G. L. Chiarotti, M. Cococcioni, I. Dabo, A. D. Corso, S. de Gironcoli, S. Fabris, G. Fratesi, R. Gebauer, U. Gerstmann, C. Gougoussis, A. Kokalj, M. Lazzeri, L. Martin-Samos, N. Marzari, F. Mauri, R. Mazzarello, S. Paolini, A. Pasquarello, L. Paulatto, C. Sbraccia, S. Scandolo, G. Sclauzero, A. P. Seitsonen, A. Smogunov, P. Umari, and R. M. Wentzcovitch, Journal of Physics: Condensed Matter **21**, 395502 (2009).
[30] G. M. Seabra, I. G. Kaplan, V. G. Zakrzewski, and J. V. Ortiz, The Journal of Chemical Physics **121**, 4143 (2004), 00018.
[31] S.-Y. Liu, K. Alnama, J. Matsumoto, K. Nishizawa, H. Kohguchi, Y.-P. Lee, and T. Suzuki, J. Phys. Chem. A **115**, 2953 (2011), 00009.
[32] N. O. Lipari and C. B. Duke, The Journal of Chemical Physics **63**, 1768 (1975).
[33] V. Coropceanu, M. Malagoli, D. A. da Silva Filho, N. E. Gruhn, T. G. Bill, and J. L. Brédas, Physical Review Letters **89**, 275503 (2002).
[34] E. Clar, J. M. Robertson, R. Schloegl, and W. Schmidt, Journal of the American Chemical Society **103**, 1320 (1981).
[35] S. Korica, A. Reinköster, M. Braune, J. Viefhaus, D. Rolles, B. Langer, G. Fronzoni, D. Toffoli, M. Stener, P. Decleva, O. Al-Dossary, and U. Becker, Surface Science **604**, 1940 (2010), 00000.
[36] D. Löffler, S. S. Jester, P. Weis, A. Böttcher, and M. M. Kappes, The Journal of Chemical Physics **124**, 054705 (2006).

[37] T. Cummins, M. Bürk, M. Schmidt, J. Armbruster, D. Fuchs, P. Adelmann, S. Schuppler, R. Michel, and M. Kappes, Chemical Physics Letters **261**, 228 (1996).
[38] P. Puschnig, E.-M. Reinisch, T. Ules, G. Koller, S. Soubatch, M. Ostler, L. Romaner, F. S. Tautz, C. Ambrosch-Draxl, and M. G. Ramsey, Physical Review B **84**, 235427 (2011).
